# Supplementary material for: Federated Learning Framework Coping with Hierarchical Heterogeneity in Cooperative ITS
Source: arXiv:2204.00215 source file (2022-07-28)
Supplement: Supplementary file 1 [file 08_appendix.tex]

Todo List:
\begin{itemize}
    \item @Rui: Proposing the idea of this paper
    \item @Rui: Implementing basic Federated Algo, FedAvg, FedProx, FedNova
    \item @Liguo: Processing the KITTI data into non-iid datasets
    \item @Liguo: Providing the training models, e.g. Yolov5, FasterRCNN, EfficientDET
    \item @Liguo: Improve the code
    \item @Rui: Rewriting the training models in federated ways
    \item @Rui: Running simulation 
    \item @Rui: Testing the results in Carla-Simulation?
    \item @Liguo: Turning parameters
    \item @Rui: Analysing results, discussing the communication and convergence speed
    \item @Rui: Writing
\end{itemize}

\begin{itemize}
    \item Proposing the federated learning for object detection model training in Cooperative Intelligent Traffic Systems
    \item Introducing the strategies for federated fashion of the camera-data in traffic scenarios considering different data skew types
    \item Analyzing and conducting the state-of-the-art methods for different data distribution 
    \item Demonstrating the federated methods in co-simulation environment considering traffic behaviors and camera model in highly-defined environment.
    \item Evaluating the simulation results with various metrics and discussing the trade-off of communication costs and algorithms' performance in vehicular networks
    \item \Crs{Providing the code online:} 
\end{itemize}

%%%%%%%%v1 
50 clients -> each client 10k images

5 client test vehicles --> 4 and 9 are missing

3 RSU: roadside unit --> Non-iid

RSU #1: 10 clients -> iid -> 1 3 5 missing 
RSU #2: 15 clients -> iid -> 2 4 6 missing
RSU #3: 20 clients -> iid -> 7 8 9 missing

50k training 
10k testing

KITTI -> 6 or 7 labels

%%%%%%%%v2 
10k as test dataset
60k in 110 clients:
    10 clients (f00000-f00009) test vehicles --> 7,8,9 are missing
    RSU #1:only 0,1 --> 10 clients (f00010-f00019)
    RSU #2:only 1,2 --> 10 clients (f00020-f00029)
    RSU #3:only 2,3 --> 10 clients (f00030-f00039)
    RSU #4:only 3,4 --> 10 clients (f00040-f00049)
    RSU #5:only 4,5--> 10 clients (f00050-f00059)
    RSU #6:only 5,6--> 10 clients (f00060-f00069)
    RSU #7:only 6,7--> 10 clients (f00070-f00079)
    RSU #8:only 7,8--> 10 clients (f00080-f00089)
    RSU #9:only 8,9--> 10 clients (f00090-f00099)
    RSU #10:only 9,0--> 10 clients (f00100-f00109)

%%%%%%%%v3 
10k as test dataset
60k in 110 clients:
6 clients (f00000-f00005) test vehicles --> 7,8,9 are missing

    RSU #1:only 0,1,2 --> 6 clients (f00010-f00015)
    RSU #2:only 1,2,3 --> 6 clients (f00020-f00025)
    RSU #3:only 2,3,4 --> 6 clients (f00030-f00035)
    RSU #4:only 3,4,5 --> 6 clients (f00040-f00045)
    RSU #5:only 4,5,6 --> 6 clients (f00050-f00055)
    RSU #6:only 5,6,7 --> 6 clients (f00060-f00065)
    RSU #7:only 6,7,8--> 6 clients (f00070-f00075)
    RSU #8:only 7,8,9--> 6 clients (f00080-f00085)
    RSU #9:only 8,9,0--> 6 clients (f00090-f00095)
    RSU #10:only 9,0,1 --> 6 clients (f00100-f00105)
    
    For each client in RSUs:
    xx0: all N0
    xx1: N0:N1:N2 = 4:1:1
    xx2: all N1
    xx3: N0:N1:N2 = 1:4:1
    xx4: all N2
    xx5: N0:N1:N2 = 1:1:4
    
%%%%%%%%v5 for KITTI:

iid dataset For testing: (The number of each labels should be the same.)

pre-train: f00000-f00005: Only Car, Pedestrian

RSU 1 (f00010-f00015): 
f00010: Only car
f00011: Only Van
f00012: Only Truck
f00013: Only Pedestrian
f00014: Only Cyclist
f00015: Only Tram
RSU 2 (f00020-f00025): Only Car
RSU 3 (f00030-f00035): Only Car
RSU 4 (f00040-f00045): Only Pedestrian
RSU 5 (f00050-f00055): Only Pedestrian

%%%%%%%%v6 for KITTI:

iid dataset For testing: (The number of each labels should be the same.)

pre-train: f00000-f00005: Only Car

RSU 1 (f00010-f00015): 
f00010: Only car and Van
f00011: Only Van and Truck
f00012: Only Truck and Pedestrian
f00013: Only Pedestrian and Cyclist
f00014: Only Cyclist and Tram
f00015: Only Tram and Car
RSU 2 (f00020-f00025): Only Car
RSU 3 (f00030-f00035): Only Car
RSU 4 (f00040-f00045): Only Pedestrian 
RSU 5 (f00050-f00055): Only Pedestrian

Todo: 
noniid explanation
performance in abstract and conclusion
key contribution
pics.

\setlength{\tabcolsep}{3pt}
\begin{table}[t]
%\bgroup\footnotesize
\begin{threeparttable}
\caption{\centering Overview of the comparison results}
\label{table:dist_est}

\begin{tabular}{C{0.5cm}C{0.5cm}C{1.6cm}C{1.6cm}C{1.6cm}C{1.6cm}}
\toprule %%%%%%%%%%%%%%%%%%
    
\multicolumn{1}{c}{ \textbf{Approaches}}  & \multicolumn{2}{c}{ \textbf{Scenario I} & \multicolumn{2}{c}}{ \textbf{Scenario II}}\\
 
  &  {Convergence Runtime}  &  {Stability}  &  {Convergence Runtime} &  {Stability} \\
 \midrule %%%%%%%%%%%%%%%%%%
 
{FedAvg}  &  {$1$}  &  {$2$}  &  {$5$} &  {$10$} \\
{FedProx}  &  {$1$}  &  {$2$}  &  {$5$} &  {$10$} \\
{HierFAVG}  &  {$1$}  &  {$2$}  &  {$5$} &  {$10$} \\
{{\myHFed} (Our Framework)}  &  {$1$}  &  {$2$}  &  {$5$} &  {$10$} \\

\bottomrule %%%%%%%%%%%%%%%%%%
\end{tabular}
    %\begin{tablenotes}
     %\small
     %\item[1] Draft versions
   %\end{tablenotes}
\end{threeparttable}
\end{table}
